# Supplementary material for: A simple method for programming and analyzing multilevel crystallization states in phase-change materials thin film
Source: arXiv:2306.17631 source file (2023-06-30)
Supplement: Supplementary file 1 [file Supplemental_Material_Taute_et_al_PCMprog_submitted.pdf]

# Supplemental Material

## A simple method for programming and analyzing multilevel crystallization states in phase-change materials thin films

*Arnaud Taute, Sadek Al-Jibouri, Capucine Laprais, Stéphane Monfray, Julien Lumeau, Antonin Moreau, Xavier Letartre, Nicolas Baboux, Guillaume Saint-Girons, Lotfi Berguiga, and Sébastien Cueff*

### Section 1: Spectroscopic ellipsometry measurements and analysis

#### Theory:

Spectroscopic ellipsometry is an optical technique used to measure the spectral amplitude (tan $\psi$) and phase ($\Delta$) of the reflected light which are related to the optical properties and microstructure of the studied sample. It is defined by:

$$\tan(\psi)\, e^{i\Delta} = R_p / R_s \qquad (S1)$$

The enabling principle of ellipsometry is that *p*- and *s*- polarized light reflect differently ($Rs \neq Rp$). We therefore measure the change of phase and polarization of light, which enables the determination of the sample's complex dielectric function ($\mathcal{E}$).

#### *Is*, *Ic* parameters:

In the case of phase-modulated ellipsometer, like the one we use, we do not measure $\psi$ and $\Delta$ directly. Instead, we measure functions of $\psi$ and $\Delta$. Here, we measure *Is* and *Ic* which are defined as:

$$Is = \sin(2\psi).\sin(\Delta), \qquad (S2)$$

$$Ic = \sin(2\psi).\cos(\Delta), \qquad (S3)$$

These trigonometric functions *Is* and *Ic* are directly related to $\psi$ and $\Delta$. They depend on the measurement conditions, in our case these above equations are only valid for the situation when the analyzer is at 45° and the modulator at 0°. Throughout this work, we directly fit the theoretical models to the *Is* and *Ic* values.

The acquired ellipsometric parameters *Is* and *Ic* of the thin film sample have been collected at an angle of 70° over a spectrum range of 260 - 2100 nm.

#### Oscillators and dispersion function to model PCMs:

The complex dielectric functions of PCM thin films and their thicknesses can be derived by fitting realistic optical models to the experimental data.

We model the optical properties of PCMs using Tauc-Lorentz oscillators, each of which corresponds to inter-band transitions in the material [39]. The equation that expresses the complex permittivity ($\varepsilon_1 + i\,\varepsilon_2$) using Tauc density of state and Lorentz oscillators is given below.

$$\tilde{\varepsilon}_{TL} = \varepsilon_{r,TL} + i.\varepsilon_{i,TL} = \varepsilon_{r,TL} + i.\varepsilon_{i,T} \times \varepsilon_{i,L} \qquad (S4)$$

The imaginary part of Tauc's dielectric function describes inter-band transitions above the band edge and Lorentz part describes inter-band transitions as dielectric oscillators. The combination of both is expressed by the equation below.

$$\varepsilon_i = \begin{cases} \sum_{i=1}^{N}\left(\frac{1}{E}\right) \times \frac{A_i.E_i.C_i.(E-E_g)^2}{(E^2-E_i^2)^2+C_i^2.E^2}, & E > E_g \\ 0, & E \leq E_g \end{cases} \quad \text{(S5)}$$

Where $A_i$ is the strength of $\varepsilon_{i,\,TL}(E)$ peak, $C_i$ represents the broadening of the peak and $E_i$ is the peak energy, where *'i'* corresponds to oscillator values. The corresponding real part of their dielectric functions, as shown below, is derived from the expression, $\varepsilon_i$ using Kramers-Kronig integration:

$$\varepsilon_r(E) = \varepsilon_r(\infty) + \sum_{i=1}^{N}\left(\frac{2}{\pi}\right).P.\int_{-\infty}^{\infty} \frac{\varepsilon_i(\xi).\xi}{\xi^2 - E^2} \quad \text{(S6)}$$

Where $\xi$ is the integration energy parameter (Cauchy's residue theorem analytics in Kramer's - Kronig integration relations) and *P* represents Cauchy's principal values.

Such a model is physically consistent and, as detailed below, each variable parameter represents a physical quantity:

- $\boldsymbol{\varepsilon_r(\infty) = \varepsilon_\infty}$ is the high frequency dielectric constant. This fitting parameter prevents $\varepsilon_1$ from converging to zero for energies below the band gap and it is generally, $\varepsilon_\infty > 1$.
- $\boldsymbol{A_i}$ (in eV) is related to the strength of the $i^{th}$ absorption peak. The subscript *'i'* refers to the number (i =1, 2 or 3) of oscillators. As $A_i$ increases, the amplitude of the peak increases and the Full Width at Half Maximum (FWHM) of that peak gets slightly larger.
- $\boldsymbol{C_i}$ (in eV) is the broadening term; it is a damping coefficient linked to the FWHM of the $i^{th}$ peak of absorption. The higher it is, the larger the peak becomes and at the same time the smaller its amplitude.
- $\boldsymbol{E_g}$ (in eV) is the optical band gap energy.

$\boldsymbol{E_i}$ (in eV) is the energy of maximum transition probability or the energy position of the peak of absorption. The subscript *'i'* refers to the number (i =1, 2 or 3) of oscillators.

## Optical Modeling of GST and fit parameters:

To model the complex permittivity of GST we used the Tauc-Lorentz model with one oscillator. Figure S1 shows the multi-layer model composed of three layers: top layer (Layer 3) being the $SiO_2$ capping layer, followed by the GST (Layer 2) and the native oxide layer (layer 1). The dispersion of silicon substrate is taken from a reference measurement. The model is then subject to free fit using least-squares curve fitting thanks to the Levenberg-Marquardt algorithm.

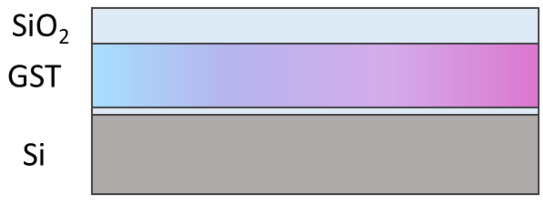


*Figure S1: Sketch of the modeled GST thin-film sample*

In the following, we display the raw *Is* and *Ic* measurements for this sample (Fig. S2), all the fits to the experimental data (Fig. S3) and all the corresponding parameters extracted from the fits (Table 1)

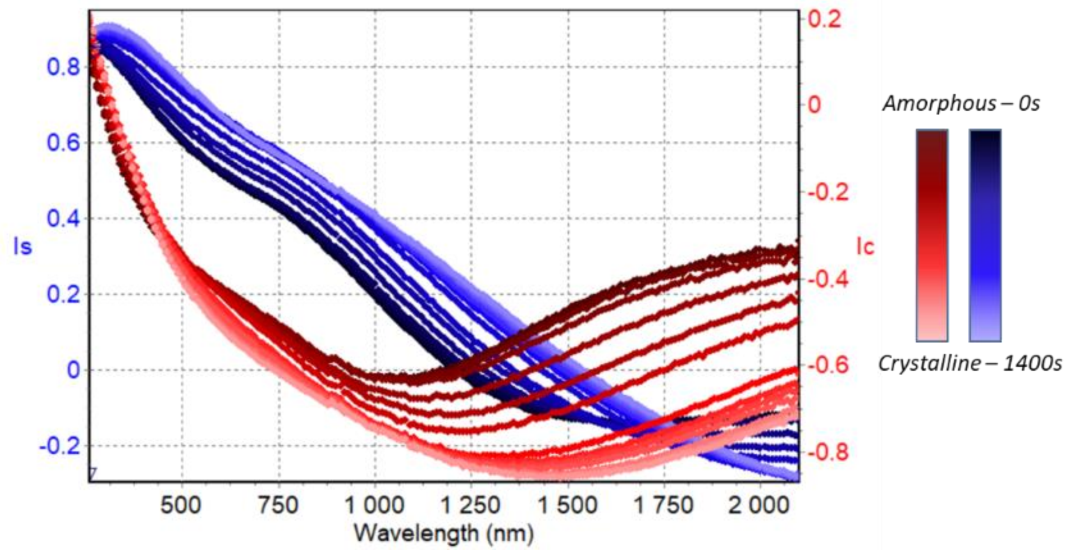


*Figure S2: Raw ellipsometry measurements Is and Ic for all partial states of crystallization of GST, measured at different time when heated at 145°C*

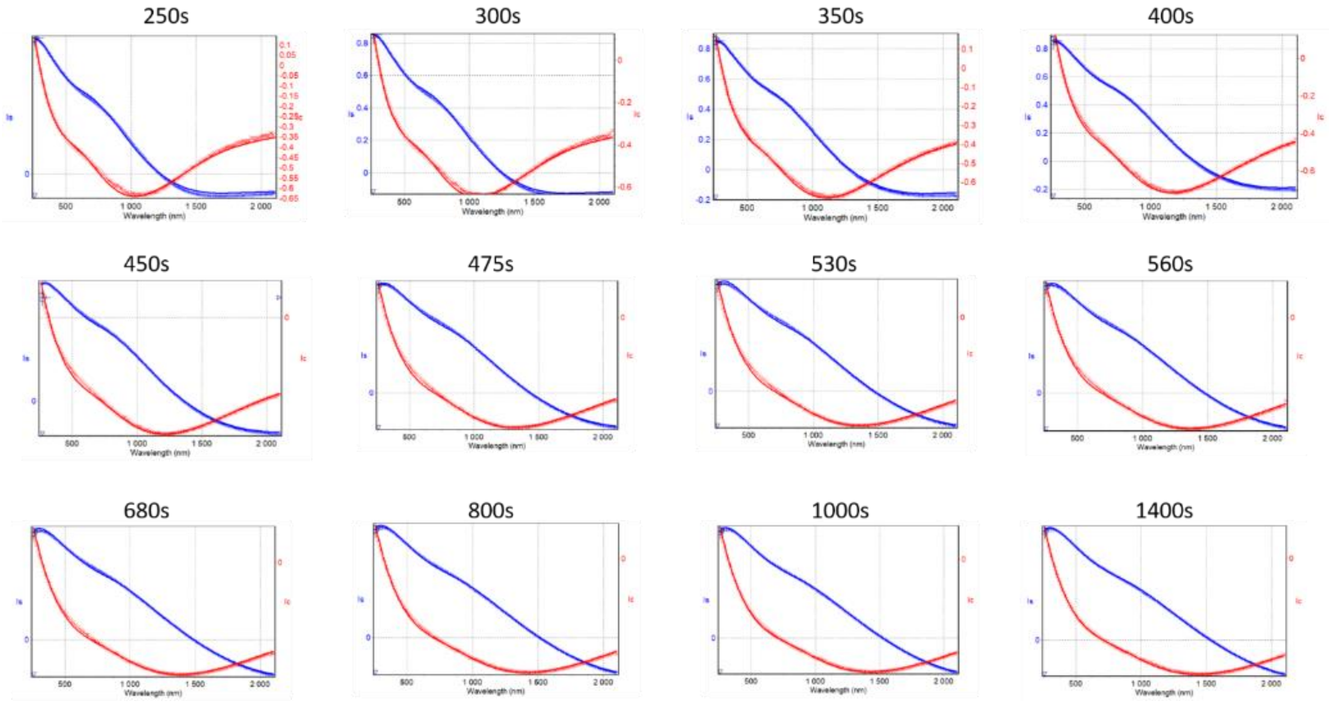


*Figure S3: Is and Ic values collected for all partial states of crystallization of GST (symbols '+' and 'x') together with their corresponding fits (lines)*

| Crystallization time (s) | 0 | 250 | 300 | 350 | 400 | 450 | 475 | 530 | 560 | 680 | 800 | 1000 | 1400 |
|---|---|---|---|---|---|---|---|---|---|---|---|---|---|
| GST Thickness (nm) | 46 | 46 | 47 | 46,5 | 46,4 | 45 | 43,8 | 44 | 43,7 | 43,7 | 43,3 | 43,26 | 43,36 |
| Eg (eV) | 0,72 | 0,705 | 0,68 | 0,62 | 0,58 | 0,55 | 0,51 | 0,5 | 0,5 | 0,496 | 0,488 | 0,484 | 0,478 |
| Eps inf | 4 | 4,2 | 4,23 | 4,7 | 5,13 | 5,22 | 5 | 4,39 | 4,55 | 4,31 | 4,3 | 4,22 | 4,4 |
| A (eV) | 129 | 127,4 | 125 | 125 | 128 | 134,6 | 150 | 153 | 159,4 | 161,6 | 169,5 | 173 | 178,5 |
| E0 (eV) | 3,05 | 3,02 | 3 | 2,78 | 2,62 | 2,37 | 2,1 | 1,99 | 1,99 | 1,96 | 1,92 | 1,9 | 1,91 |
| C (eV) | 4,56 | 4,52 | 4,5 | 4,2 | 4 | 3,61 | 3,15 | 2,93 | 2,95 | 2,88 | 2,83 | 2,8 | 2,82 |

*Table 1: Fit parameter values obtained for all crystallization states of GST*

Optical Modeling of $Sb_2S_3$ and fit parameters:

To model the complex permittivity of $Sb_2S_3$ thin films we used the Tauc-Lorentz model with three oscillators. Figure S4 shows the multi-layer model composed of three layers: top layer (Layer 3) being the $SiO_2$ capping layer, followed by the $Sb_2S_3$ (Layer 2) and an effective medium approximation layer (EMA - layer 1). The dispersion of silicon substrate is taken from a reference measurement. The model is then subject to free fit using least-squares curve fitting thanks to the Levenberg-Marquardt algorithm. The EMA layer is used to account for the early stages of crystallization of $Sb_2S_3$ at the interface, as well as the progressive growth of crystals from this interface and the concomitant disappearance of native $SiO_2$. Indeed, as crystallization initiates at nucleation centers, it is more likely to start at the interface with the substrate. This EMA, although requiring more in-depth studies, proved to be a very efficient and reliable means to enable excellent fits for all states of $Sb_2S_3$ and to capture the progressive crystallization in the layer.

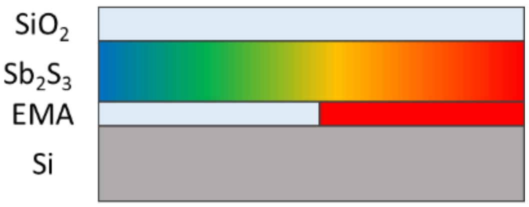


*Figure S4: Sketch of the modeled $Sb_2S_3$ thin-film sample*

In the following, we display the raw *Is* and *Ic* measurements for this sample (Fig. S5), all the fits to the experimental data (Fig. S6) and all the corresponding parameters extracted from the fits (Table 2)

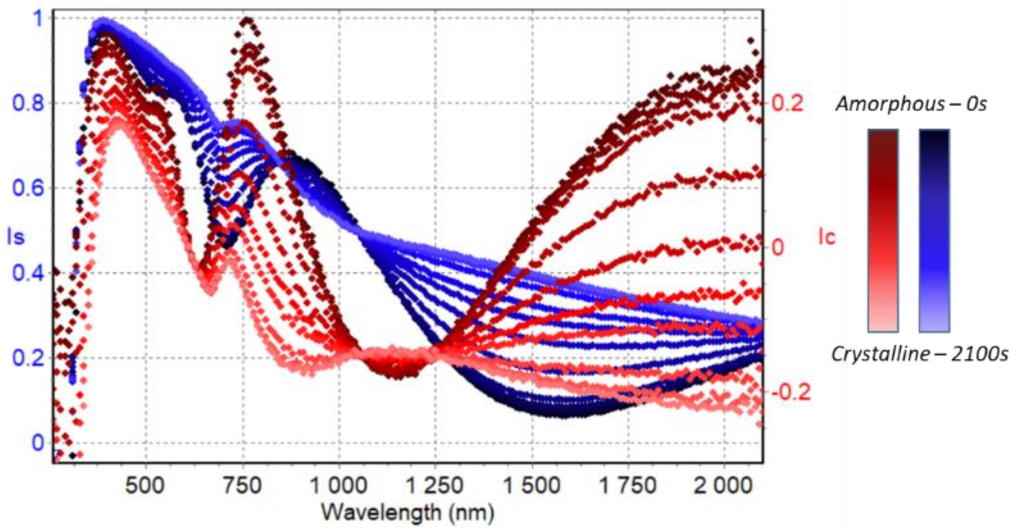


*Figure S5: Raw ellipsometric measurements Is and Ic for all partial states of crystallization of $Sb_2S_3$ at different times when hetaed at 260°C*

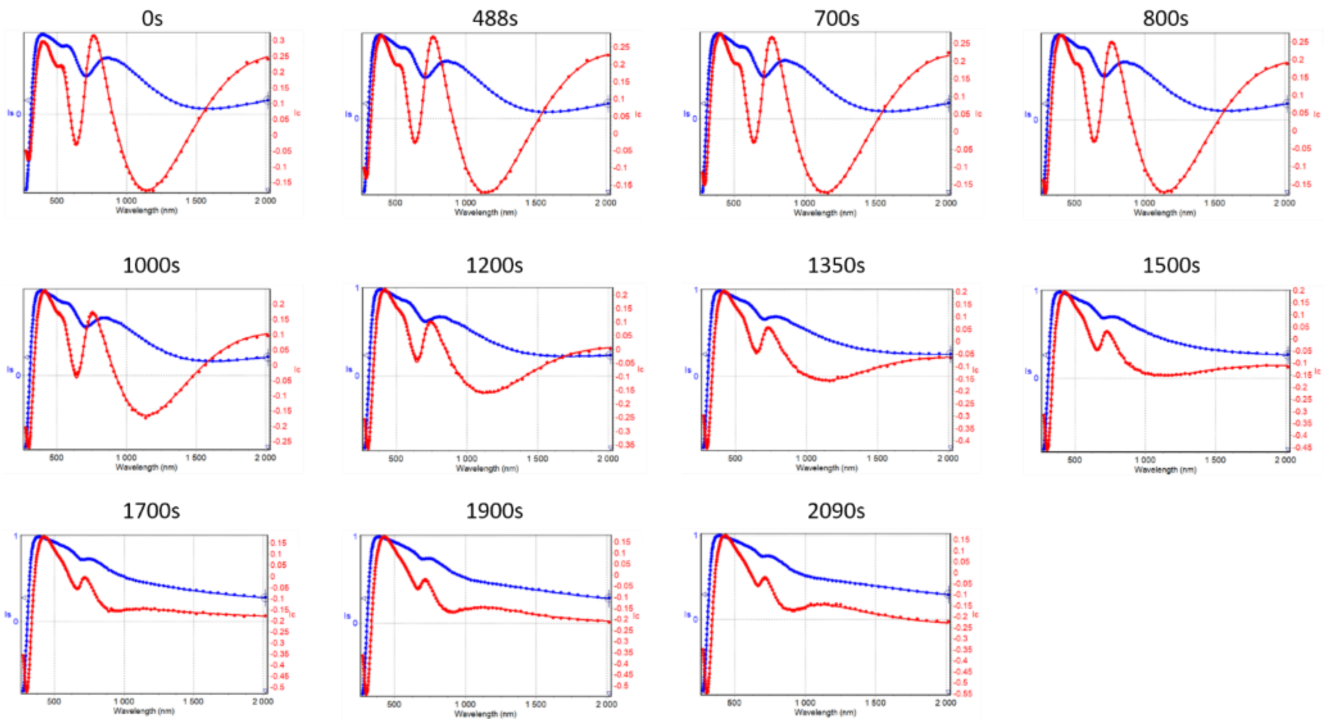


*Figure S6: Is and Ic values collected for all partial states of crystallization of $Sb_2S_3$ (circles) together with their corresponding fits (lines)*

| Crystallization time (s) | 0 | 488 | 700 | 800 | 1000 | 1200 | 1350 | 1500 | 1700 | 1900 | 2090 |
|---|---|---|---|---|---|---|---|---|---|---|---|
| Thickness Sb2S3 | 184 | 176 | 174 | 170 | 175 | 167 | 161 | 157 | 152 | 129 | 166 |
| Thickness interface | 2,8 | 7,7 | 7,8 | 8 | 8,2 | 15,4 | 16,9 | 17,8 | 18 | 41 | 0 |
| Interfacial Sb2S3 % | 0 | 54,5 | 55 | 54 | 100 | 100 | 100 | 100 | 100 | 100 | 100 |
| Eg | 1,69 | 1,61 | 1,63 | 1,64 | 1,59 | 1,28 | 1,23 | 1,23 | 1,24 | 1,18 | 1,3 |
| Eps inf | 2,69 | 2,66 | 2,6 | 2,6 | 2,44 | 2,65 | 2,55 | 2,66 | 2,66 | 2,61 | 2,8 |
| A1 | 18,5 | 10 | 7,7 | 6 | 14,8 | 9,6 | 16,8 | 13,1 | 12,85 | 13,17 | 208 |
| E1 | 5 | 5 | 5 | 4,9 | 4,95 | 4,9 | 4,95 | 4,9 | 4,9 | 4,9 | 2,9 |
| C1 | 1,95 | 1,51 | 1,22 | 1,03 | 1,56 | 1,1 | 1,67 | 1,3 | 1,34 | 1,49 | 3,5 |
| A2 | 25,2 | 19,2 | 20 | 9,8 | 79,9 | 14,7 | 25,4 | 29,6 | 48 | 46,5 | 7,5 |
| E2 | 2,76 | 2,83 | 2,83 | 2,75 | 3 | 2,7 | 2,7 | 2,67 | 2,69 | 2,69 | 3,56 |
| C2 | 1,12 | 1,09 | 1,14 | 0,86 | 2,36 | 1,13 | 1,19 | 1,28 | 1,38 | 1,36 | 0,58 |
| A3 | 46,7 | 58,5 | 66,9 | 87,5 | 19 | 56,5 | 41,3 | 45,7 | 39,2 | 37,3 | 1,14 |
| E3 | 3,69 | 3,64 | 3,65 | 3,5 | 3,7 | 3,53 | 3,5 | 3,49 | 3,5 | 3,42 | 1,92 |
| C3 | 2,05 | 2,3 | 2,46 | 2,6 | 1,47 | 1,95 | 1,57 | 1,6 | 1,5 | 1,46 | 0,09 |

*Table 2: Fit parameter values obtained for all crystallization states of $Sb_2S_3$*

## Section 2: Evolution of the refractive index and Is as a function of crystalline fraction

In this section we justify our choice of using normalized values of *Is* parameter as a probe of the crystalline fraction of PCM within an amorphous host of the same material.
We first consider the effective medium theory, and in particular the Bruggeman formula that was used in the theoretical part of the paper.

$$f\frac{\varepsilon_{r1}-\varepsilon_B}{\varepsilon_{r1}+2\varepsilon_B}+(1-f)\frac{\varepsilon_{r2}-\varepsilon_B}{\varepsilon_{r2}+2\varepsilon_B}=0 \qquad \text{(Eq. S1)}$$

Where $\varepsilon_{r1}$ and $\varepsilon_{r2}$ are the permittivities of the two materials, $\varepsilon_B$ is the effective permittivity of the mixed medium and *f* is the fill fraction.
In this theory, when the two materials do not present large permittivity contrasts, the resulting effective permittivity linearly scales with the fill fraction. In figure S7, we display how the complex refractive index evolves against the crystalline fraction for both GST and $Sb_2S_3$

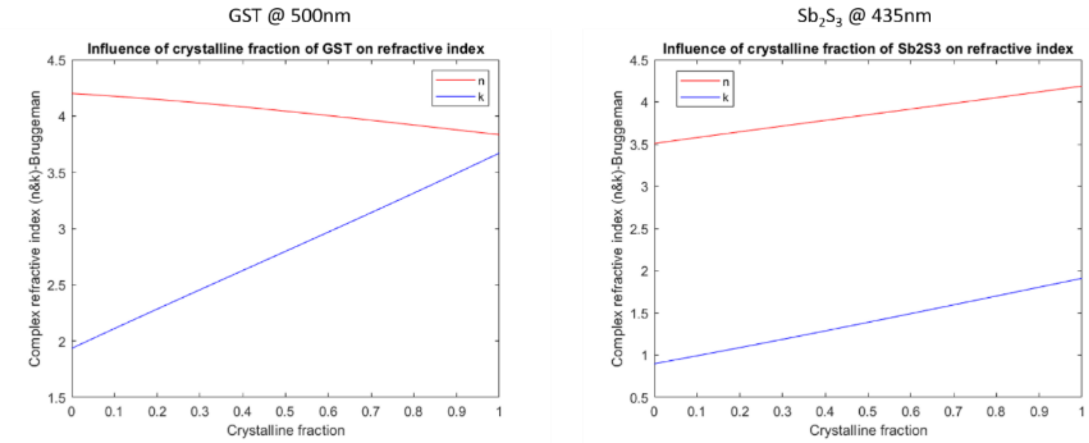


*Figure S7: Evolution of refractive index and extinction coefficient as a function of the crystalline fraction for both GST and $Sb_2S_3$*

We see that in the two cases both the refractive index and the extinction coefficient follow a linear trend, hence showing that the evolution of the complex effective refractive index should scale linearly against the crystalline fraction.

We now want to confirm that trend in the particular case of thin-films of PCMs on top of Silicon. As displayed in figure S8, the *Is* parameter as a function of the crystalline fraction of both GST and $Sb_2S_3$ are not necessarily linear throughout the wavelength range, but show monotonic quasi-linear trends for the wavelengths chosen to monitor the crystallization in this work (respectively 500nm and 435nm). Future works could include refined linearization procedures to optimize the precision, but for the sake of simplicity, we have decided here to consider this small non-linearity a second order effect. This weak deviation has a negligible qualitative impact on the obtained results and most importantly does not change any of the conclusions drawn in this work.

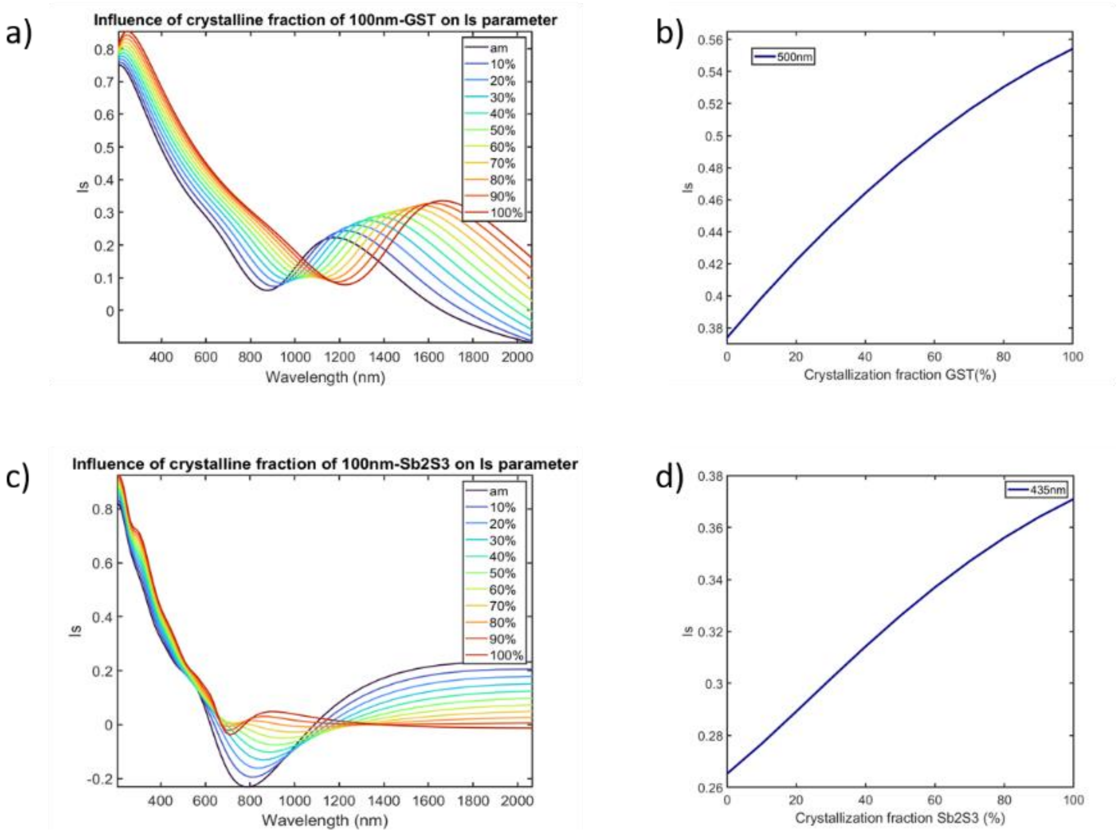


*Figure S8: Influence of the crystalline fraction of PCM on the evolution of the Is parameter. a) 100-nm-thick layer of GST on silicon, for all wavelengths (a) and at the measured wavelength of 500nm (b); c) 100-nm-thick $Sb_2S_3$ layer on silicon, for all wavelengths (c) and at the measured wavelength of 435 nm*
